# Supplementary material for: Sharp Analysis for Nonconvex SGD Escaping from Saddle Points
Source: arXiv:1902.00247 source file (2019-06-04)
Supplement: Supplementary file 2 [file appendix_part2_stage1.tex]

\pb\section{Deferred Proofs of Part \mbox{II}: Faster Descent}
\red{Filtrations are all wrong!}
We prove our the following theorem:
\begin{theorem}\label{faster descent}
	For  Algorithm \ref{algo:two-phase SGD} with parameter set in \eqref{parametersetting},  for any  $j\geq 0$, \red{given $\cF^{\cK-1}$,} if $\x^k$ moves out of  $\cB(\x^{0}, B)$ in $K_0$ iteration then with probability at least $1-\frac{2}{3}p_3$, we have
\begin{eqnarray}
f\left(\x^{\cK(j+1)}\right) \leq f\left(\x^{0}\right) - \frac{B^2}{7\eta K_0}.
\end{eqnarray}	
\end{theorem}

 We use $0$ to denote the iteration index at beginning for $j$-times exiting the $B$-neighborhood (Refer Step \ref{denote ck} in Algorithm \ref{algo:two-phase SGD}), and $\sK(j)$ be  the  time that $\x^k$ exits  $\cB\left(\x^{0},B\right)$, i.e.,	
	\begin{eqnarray}\label{define of sk}
	\sK(j)   = \min\left(\inf_{k\geq 0 }( \|\x^{k} - \x^{0} \|\geq B), ~~ \cK\le K_0-1\right).
	\end{eqnarray}	
Because $\x^{k+1}$ is measurable on $\cF^k$,  $\sK(j)$ is a stopping time.	And if Algorithm\ref{algo:two-phase SGD} has not stopped at $j$, we  have  $\cK(j+1)=\sK(j)+1$.  W.L.O,G, if our analysis only focuses on the dynamic in $\cB(\x^{0}, B)$,  we   use $0$ and $\sK$ to denote $0$ and $\sK(j)$, respectively.

\pb\subsection{Definition and Preliminary}
When given $\cF^{\cK-1}$,  $\x^{0}$, $\nabla^2 f(\x^{0})$,  and $\nabla^2 f(\x^{0})$  are measurable.  In the following,  we use $\bH$ to denote $\nabla^2 f(\x^{0})$ and let $\cS$ be the subspace spanned by all eigenvectors of $\bH$ whose eigenvalue is greater than $0$, and $\cS\bot$ denotes the complement space. We denote $\cP_{\cS\bot} \in \RR^{d\times d }$ and $\cP_{\cS}\in \RR^{d\times d }$ as the projection matrices on to the space of $\cS$ and $\cS\bot$, respectively.  Also  let  the full SVD decomposition of $\bH$ as $\mathbf{V}\sum \mathbf{V}^T$. We introduce $\bH_{\cS} = \mathbf{V}\sum_{(\lambda_i >0)}\mathbf{V}^T$, and  $\bH_{\cS\bot} = \mathbf{V}\sum_{(\lambda_i \leq0)}\mathbf{V}^T$. Then  $\bH = \bH_{\cS} + \bH_{\cS\bot}$.

 Let $\uu^k = \cP_{\cS} \left(\x^k - \x^{0}\right)$, and $\vv^k = \cP_{\cS\bot}\left(\x^k - \x^{0}\right) $. We can decompose the update equation of Step \ref{update1} as: 
\begin{eqnarray}
\uu^{k+1} &=& \uu^{k} - \eta \cP_{\cS}\nabla f\left(\x^k\right) - \eta  \cP_{\cS}\bxi^k. \label{update u}\\
\vv^{k+1}  &=& \vv^{k} - \eta \cP_{\cS\bot}\nabla f\left(\x^k\right) - \eta  \cP_{\cS\bot}\bxi^k,  \label{update v}
\end{eqnarray}
with $k \geq 0$. And $\uu^{0} = \mathbf{0}$, $\vv^{0} = \mathbf{0}$.
Let $g(\x)$  be the quadratic approximation of $f(\x) - f(\x^{0})$ at $\x^{0}$, i.e.
\begin{eqnarray}
g(\x) &=&  \left[\nabla f(\x^{0})\right]^\bT\left(\x - \x^{0}\right) +  \frac{1}{2}\left[\x - \x^{0}\right]^\bT \bH \left[\x - \x^{0}\right] \\
&=&  \left[\nabla f(\x^{0})\right]^\bT\left[\cP_{\cS} \left(\x - \x^{0}\right) + \cP_{\cS\bot} \left(\x - \x^{0}\right)\right]+ \frac{1}{2}\left[\cP_{\cS} \left(\x - \x^{0}\right)\right]^\bT \bH \left[\cP_{\cS} \left(\x - \x^{0}\right)\right]\notag\\
&& +  \frac{1}{2}\left[\cP_{\cS\bot} \left(\x - \x^{0}\right)\right]^\bT \bH \left[\cP_{\cS\bot} \left(\x - \x^{0}\right)\right]\notag\\
&=& \left[\cP_{\cS} \nabla f(\x^{0})\right]^\bT\left[\cP_{\cS} \left(\x - \x^{0}\right)\right]+ \left[\cP_{\cS\bot} \nabla f(\x^{0})\right]^\bT\left[\cP_{\cS\bot} \left(\x - \x^{0}\right)\right]\notag\\
&& + \frac{1}{2}\left[\cP_{\cS} \left(\x - \x^{0}\right)\right]^\bT \bH_{\cS} \left[\cP_{\cS} \left(\x - \x^{0}\right)\right] +  \frac{1}{2}\left[\cP_{\cS\bot} \left(\x - \x^{0}\right)\right]^\bT \bH_{\cS\bot} \left[\cP_{\cS\bot} \left(\x - \x^{0}\right)\right], \notag
\end{eqnarray} 
where in the last equality  we use $\cP^2_{\cS} = \cP_{\cS}$ and $\cP^2_{\cS\bot} = \cP_{\cS\bot}$, because $\cP_{\cS}$ and $\cP_{\cS\bot}$ are projection matrices.
Define two auxiliary functions $g_{\cS}:\cS\to \RR$ and  $g_{\cS\bot}:\cS\bot\to \RR$ satisfying:
\begin{eqnarray}
g_{\cS}(\uu) =   \left[\cP_{\cS}\nabla f\left(\x^{0}\right)\right]^\bT\uu +  \frac{1}{2}\uu^T \bH_{\cS} \uu,
\end{eqnarray}
and 
\begin{eqnarray}
g_{\cS\bot}(\vv) =   \left[\cP_{\cS\bot}\nabla f\left(\x^{0}\right)\right]^\bT\vv +  \frac{1}{2}\vv^T \bH_{\cS\bot} \vv .
\end{eqnarray}
So if  $\uu = \cP_{\cS} \x$ and $\vv = \cP_{\cS\bot} \x$,  we have
\begin{eqnarray}
g(\x) = g_{\cS}(\uu) + g_{\cS\bot}(\vv).
\end{eqnarray} 
For clarify,  we denote $\nabla_{\uu} f(\x^k) = \cP_{\cS}\nabla f(\x^k)$, and  $\nabla_{\vv} f(\x^k)  = \cP_{\cS\bot}\nabla f(\x^k)$, respectively. Similarly, let $\bxi_{\uu}^k = \cP_{\cS}\bxi^k$, and  $\bxi_{\vv}^k = \cP_{\cS\bot}\bxi^k$.  The following Lemma is basic to obtain our result.

\pb
\begin{lemma}
Given $\cF^{\cK-1}$, for any $\x$, if $\left\| \x - \x^{0}\right\| \leq B$, then
	\begin{eqnarray}\label{basic1}
	\|\nabla f(\x) - \nabla g(\x) \| \leq \rho B^2/2.
	\end{eqnarray}
  For any symmetric matrix $\A$, and $0\leq a \leq \frac{1}{\|\A\|_2}$,  we have
  \begin{eqnarray}\label{basic2}
  \left\|(\I - a \A)^i \A (\I - a \A)^j\right\|_2 \leq \frac{1}{a(i+j+1)}.
  \end{eqnarray}
\end{lemma}

\pb
\begin{proof}
	For \eqref{basic1}, we have
	\begin{eqnarray}
	&&\left\|\nabla f(\x) - \nabla g(\x) \right\|\notag\\
	&=&\left\|\nabla f(\x) - \nabla f(\x^{0}) - \bH (\x - \x^{0}) \right\|\notag\\
	&=&\left\|\left(\int_{0}^1 \nabla^2 f(\x^{0} + \theta (\x - \x^0)) d_{\theta} - \bH\right)  \left(\x - \x^{0}\right) \right\|\notag\\
	&\overset{a}\leq& \left\|\left(\int_{0}^1  \rho \theta \left\| \x - \x^0\right\| d_{\theta} \right) \right\|   \left\|\x - \x^{0}\right \|\notag\\
	&\leq& \rho B^2/2
	\end{eqnarray} 
	where in $\overset{a}\leq$, we use Assumption \ref{a4} that $f(\x)$ has $\rho$-Lipschitz continuous Hessian.
	
	\eqref{basic2} is from \cite{jin2017escape}. To prove it, suppose the eigenvalue of $\{\A\}$  is $\{\lambda_l\}$, thus the  eigenvalue of $(\I - a \A)^i\bH (\I - a \A)^{j}$ is $\{\lambda_l (1 - a \lambda_l)^{i+j} \}$. For the function of $\lambda (1 - a \lambda)^{i+j}$, we can compute out its derivative as $ (1 - a\lambda)^{i+j} - (i+j)a \lambda (1 - a \lambda)^{i+j-1}$. Then with simple analysis, we can find that  the maximal point is obtained only at $\frac{1}{(1+i+j)a}$. Thus we have
\begin{eqnarray}
\left\|(\I - a \A)^i \A (\I - a \A)^j\right\|_2 \leq \frac{1}{(1+j+i)a} \left(1 - \frac{1}{1+j+i}\right)^{j+i} \leq \frac{1}{(1+j+i)a}.
\end{eqnarray}
\end{proof}

\pb\subsection{Analysis on Quadratic  Approximation}\label{quadratic}
As have been introduced  before, our main technique to obtain a faster $\tO(\ep^{-3.5})$ convergence rate is by separately analyzing  the two quadratic  approximations: $g_{\cS}(\cdot)$, and $g_{\cS\bot}(\cdot)$. The following two Lemmas describe the properties of $g_{\cS}(\cdot)$, and $g_{\cS\bot}(\cdot)$, respectively.

\pb
\begin{lemma}\label{analysis on uu}
Given $\cF^{\cK-1}$, let $\x^{k}$ is updated by Step \ref{update rule} in Algorithm \ref{algo:two-phase SGD} with hyper-parameters set in \eqref{parametersetting},   with probability at least $1 - p_3/4$,  we have
\begin{eqnarray}\label{uu end4}
\!\!\!\!\!\!g_{\cS}(\uu^{\sK+1})  - g_{\cS} (\uu^{0})\leq-\frac{25\eta\sum_{k=0}^{\sK}\left\|  \nabla  g_{\cS} \left(\y^k\right)\right\|^2  }{32} +4\eta \sigma^2 \left( 1+3\log(K_0)\right) \log(48/p_3) + \eta \rho^2 B^4 K_0.
\end{eqnarray}
\end{lemma}

\pb
\begin{lemma}\label{analysis on vv}
	Given $\cF^{\cK-1}$, let $\x^{k}$ is updated by Step \ref{update rule} in Algorithm \ref{algo:two-phase SGD} with hyper-parameters set in \eqref{parametersetting},    we have
	\begin{eqnarray}\label{vv end5}
g_{\cS\bot}(\vv^{\sK+1}) \leq g_{\cS\bot}(\vv^{0})  -  \sum_{k =0}^{\sK}  \eta\< \nabla g_{\cS\bot}\left(\vv^{k}\right),  \bxi_{\vv}^k\>  - \frac{7\eta}{8}\sum_{k =0}^{\sK}  \left\|  \nabla g_{\cS\bot}\left(\x^{k}\right)  \right\|^2 + \frac{\rho^2 B^4 \eta K_0}{2}.
	\end{eqnarray}
\end{lemma}
\begin{remark}
 Notice that the terms $\eta\< \nabla g_{\cS\bot}(\vv^{k}) ,  \bxi_{\vv}^k\>$ with $k$ from $0$ to $\sK$ in 	Lemma \ref{analysis on vv} cannot be   treated  as zero when taken expectation. This is because our analysis relies on the condition that $\x$ exits the $B$-neighborhood in $K_0$ iterations, i.e. $\| \x^{\sK+1}-\x^{0}\|\geq B$, which is not predictable   on  $\cF^{\cK-1}$. 
We leave the details to  tackle the problem in the next subsection.
\end{remark}

\pb
\begin{proof}[Proofs of Lemma \ref{analysis on uu}]
 We  consider an auxiliary trajectory, which performs update as:
\begin{eqnarray}\label{y update}
\y^{k+1} = \y^k - \eta \nabla g_{\cS}\left(\y^k\right), \quad k\geq 0.
\end{eqnarray}
and $\y^{0} = \uu^{0}$.   Clearly, $\y^{k}$ preforms Gradient Decent on $ g_{\cS} (\cdot)$,  which is deterministic given $\cF^{0}$. We  study the property of $\y^{\sK}$ and obtain the following standard results:
\begin{itemize}
	\item Because $g_{\cS}(\cdot)$ has $L$-Lipschitz continuous gradient ($\| \bH_{\cS}\|_2 \leq L$), we have
	\begin{eqnarray}\label{update y}
	&&g_{\cS}\left(\y^{k+1}\right)\notag\\
	&\leq&g_{\cS}\left(\y^{k}\right) + \< \nabla g_{\cS}\left(\y^{k}\right), \y^{k+1} - \y^k  \> +  \frac{L}{2}\left\|\y^{k+1} - \y^{k}\right\|^2\notag\\
	&\overset{\eqref{y update}}{=}& g_{\cS} \left(\y^k\right)  - \eta \left(1 - \frac{L\eta}{2}\right)\left\| \nabla g_{\cS}\left(\y^{k}\right)\right\|^2.
	\end{eqnarray}
	\item By telescoping \eqref{update y} from $0$ to $\sK$, we have
	\begin{eqnarray}\label{uu end2}
	g_{\cS}\left(\y^{\sK+1}\right)&\leq& g_{\cS}\left(\y^{0}\right) - \eta\left(1 - \frac{L\eta}{2}\right) \sum_{k =0}^{\sK}\left\| \nabla g_{\cS}\left(\y^{k}\right)\right\|^2\notag\\
	& \overset{L \eta \leq \frac{1}{16}}{\leq}& g_{\cS}\left(\y^{0}\right) - \frac{31\eta}{32} \sum_{k =0}^{\sK}\left\| \nabla g_{\cS}\left(\y^{k}\right)\right\|^2.
	\end{eqnarray}
\end{itemize}
\end{proof}

\pb
Now we  bound the difference between $\uu^\sK $ and $\y^{\sK}$. Let $\z^{k} = \uu^k - \y^k$ be the difference iteration, we have
\begin{eqnarray}\label{update of z}
\z^{k+1} &=& \z^{k} - \eta \left(\nabla g_{\cS}\left(\uu^k\right)-\nabla g_{\cS}\left(\y^k\right)\right) -  \eta\left(\nabla_{\uu}f\left(\x^k\right) - \nabla g_{\cS}\left(\uu^k\right)\right) - \eta \bxi^k_{\uu}\notag\\
&=& (\I - \eta \bH_{\cS} )\z^k - \eta\left(\nabla_{\uu}f\left(\x^k\right) - \nabla g_{\cS}\left(\uu^k\right)\right)- \eta \bxi^k_{\uu}, \quad k\geq 0.
\end{eqnarray}
And $\z^{0} = \mathbf{0}$.

The following Lemma concludes the property of $\z^{\sK+1}$.
\begin{lemma}\label{zz}
	With probability at least  $1 - p_3/6$, we have
	\begin{eqnarray}\label{z4}
	\left\| \z^{\sK+1}\right\|\leq \frac{3B}{32}.
	\end{eqnarray}
	and 
	\begin{eqnarray}\label{z5}
	\left(\z^{\sK+1}\right)^\bT \bH_{\cS} \left(\z^{\sK+1}\right) \leq   8\sigma^2 \eta \left(\log(K_0)+1\right) \log(48/p_3) + \eta \rho^2 B^4 K_0.
	\end{eqnarray}
\end{lemma}

\pb
\begin{proof}[Proofs of Lemma \ref{zz}]
 We can obtain the general solution of \eqref{update of z} as
	\begin{eqnarray}
	\z^k =  - \sum_{j =0}^{k-1}\eta (\I - \eta \bH_{\cS})^{k -1- j} \bxi_{\uu}^j  - \eta \sum_{j =0}^{k-1} (\I - \eta \bH_{\cS})^{k-1 - j} \left(\nabla_{\uu}f\left(\x^j\right) - \nabla g_{\cS}\left(\uu^j\right)\right), \quad k\geq 0.
	\end{eqnarray}
	
By triangle inequality, we have 
	\begin{eqnarray}\label{z3}
	\left\|\z^{\sK+1} \right\| \leq   \left\| \sum_{j =0}^{\sK}\eta (\I - \eta \bH_{\cS})^{\sK - j} \bxi_{\uu}^j\right\| + \left\| \eta \sum_{j =0}^{\sK} (\I - \eta \bH_{\cS})^{\sK - j} \left(\nabla_{\uu}f\left(\x^j\right) - \nabla g_{\cS}\left(\uu^j\right)\right) \right\|.
	\end{eqnarray}
	For the first term in the right hand of \eqref{z3}, because for all $0\leq j\leq\sK$, we have 
	\begin{eqnarray}\label{z1}
	\left\| \eta (\I - \eta \bH_{\cS})^{\sK - j} \bxi_{\uu}^j\right\| \leq \eta \sigma.
	\end{eqnarray}
	 By the Vector-Martingale Concentration Inequality in Subsection \ref{123}, we have with probability $1 - p_3/12$,  
	\begin{eqnarray}\label{probability1}
	\left\| \sum_{j =0}^{\sK}\eta (\I - \eta \bH_{\cS})^{\sK - j} \bxi_{\uu}^j\right\|\leq 2\eta \sigma\sqrt{ (\sK - 0 ) \log(48/p_3)} \leq 2\eta \sigma\sqrt{ K_0 \log(12/p_3)}\overset{\eqref{parametersetting}}{\leq} \frac{B}{16}.
	\end{eqnarray}

	For the  second term in the right hand of \eqref{z3},  we  have 
	\begin{eqnarray}\label{z2}
	&& \left\| \eta \sum_{j =0}^{\sK} (\I - \eta \bH_{\cS})^{\sK - j} \left(\nabla_{\uu}f\left(\x^j\right) - \nabla g_{\cS}\left(\uu^j\right)\right) \right\|\notag\\
	&\leq&\eta \sum_{j =0}^{\sK} \left\|\nabla f\left(\x^j\right) - \nabla g\left(\uu^j\right)  \right\|\overset{\eqref{basic1}}{\leq }  \frac{\rho\eta B^2 K_0}{2} \overset{\eqref{parametersetting}}{\leq} \frac{B}{32}.
	\end{eqnarray}

	Substituting \eqref{probability1} and \eqref{z2} into \eqref{z3}, we obtain \eqref{z4}.

	To prove \eqref{z5}, using the fact that  $(\a + \b)^\bT \A (\a+ \b) \leq 2 \a^{\bT}\A \a +2 \b^{\bT}\A \b  $ holds for  any  symmetry positive  definite matrix $\A$, we have
	\begin{eqnarray}\label{zend1}
	&&\left(\z^{\sK+1}\right)^\bT \bH_{\cS} \left(\z^{\sK+1}\right) \\
	&\leq& 2\eta^2 \left(\sum_{j =0}^{\sK} (\I - \eta \bH_{\cS})^{\sK - j} \bxi_{\uu}^j \right)^\bT \bH_{\cS} \left(\sum_{j =0}^{\sK} (\I - \eta \bH_{\cS})^{\sK - j} \bxi_{\uu}^j \right)\notag\\
	&&+ 2\eta^2 \left( \sum_{j =0}^{\sK} (\I - \eta \bH_{\cS})^{\sK - j} \left(\nabla_{\uu}f\left(\x^j\right) - \nabla g_{\cS}\left(\uu^j\right)\right)\right)^{\bT}\bH_{\cS} \left( \sum_{j =0}^{\sK} (\I - \eta \bH_{\cS})^{\sK - j} \left(\nabla_{\uu}f\left(\x^j\right) - \nabla g_{\cS}\left(\uu^j\right)\right)\right)\notag\\
	&=& 2\left\| \eta\left(\sum_{j =0}^{\sK} \bH^{1/2}_{\cS}(\I - \eta \bH_{\cS})^{\sK - j} \bxi_{\uu}^j \right)   \right\|^2\notag\\
	&& + 2\eta^2 \sum_{j =0}^{\sK}\sum_{l =0}^{\sK}\left(\nabla_{\uu}f\left(\x^j\right) - \nabla g_{\cS}\left(\uu^j\right)\right)^\bT (\I - \eta \bH_{\cS})^{\sK - j}\bH_{\cS}(\I - \eta \bH_{\cS})^{\sK - l}\left(\nabla_{\uu}f\left(\x^j\right) - \nabla g_{\cS}\left(\uu^j\right)\right)\notag\\
	&\overset{\eqref{basic1}}{\leq}&2\left\| \eta\left(\sum_{j =0}^{\sK}  \bH^{1/2}_{\cS}(\I - \eta \bH_{\cS})^{\sK - j} \bxi_{\uu}^j \right)   \right\|^2 + 2\eta^2\frac{\rho^2 B^4}{4}\sum_{j =0}^{\sK}\sum_{l=0}^{\sK} \left\|  (\I - \eta \bH_{\cS})^{\sK - j}\bH_{\cS}(\I - \eta \bH_{\cS})^{\sK - l} \right\|_2.\notag
	\end{eqnarray}
	
For 	the first term in the right hand $\eqref{zend1}$,   for any $0\leq j \leq\sK$, we have
	\begin{eqnarray}
	&&\left\|\eta\left( \bH^{1/2}_{\cS}(\I - \eta \bH_{\cS})^{\sK - j} \bxi_{\uu}^j \right)\right\|^2\notag\\
	&  \leq&  \eta^2\|\bxi_{\uu}^j\|  \left\| (\I - \eta  \bH_{\cS})^{\sK - j}  \bH^{1/2}_{\cS}  (\I - \eta  \bH_{\cS})^{\sK - j}\right \|_2\|\bxi_{\uu}^j  \| \overset{\eqref{basic2}} {\leq}  \frac{\eta\sigma^2}{1+2 (\sK-j)},
	\end{eqnarray}
	then by  the Vector-Martingale Concentration Inequality in Subsection \ref{123}, we have with probability $1 - p_3/12$
	\begin{eqnarray}\label{probability2}
	&&\left\| \eta\left(\sum_{j =0}^{\sK} \cH^{1/2}(\I - \eta \bH_{\cS})^{- j} \bxi_{\uu}^j \right)   \right\|^2 \leq   4 \eta \sigma^2\log(48/p_3) \sum_{j=0}^{\sK} \frac{1}{1+2(\sK-j)}   \notag\\
	&\leq& 4\sigma^2 \eta   \log(48/p_3)\sum_{j= 0}^{K_0} \frac{1}{1+j}   \leq 4\sigma^2 \eta \left(\log(K_0)+1\right) \log(48/p_3).
	\end{eqnarray}
	
	For the second term in the right hand $\eqref{zend1}$,  we have
	\begin{eqnarray}\label{z7}
	&&\eta^2\frac{\rho^2 B^4}{4}\sum_{j =0}^{\sK}\sum_{l =0}^{\sK} \left\|  (\I - \eta \bH_{\cS})^{\sK - j}\bH(\I - \eta \bH_{\cS})^{\sK - l} \right\|_2 \notag\\
	&\leq&\eta\frac{\rho^2 B^4}{4} \sum_{j =0}^{\sK}\sum_{j =l}^{\sK}  \frac{1}{1+ (\sK - j)+(\sK - l) }\leq\eta\frac{\rho^2 B^4}{4} \sum_{j =0}^{K_0-1}\sum_{l =0}^{K_0-1}  \frac{1}{1+ j +l} \notag\\
	&=&\eta\frac{\rho^2 B^4}{4} \sum_{j=0}^{2(K_0-1)} \frac{\min(1+j, 2K_0-1 - j)}{1+j}\leq \frac{\eta\rho^2 B^4 K_0}{2}.
	\end{eqnarray}
	Substituting \eqref{probability2} and \eqref{z7} into \eqref{zend1}, we obtain \eqref{z5}.
\end{proof}

\pb
\begin{proof}[Proof of Lemma \ref{analysis on uu}]
 Let $\y^* = \argmin_{\y} g_{\cS} (\y)$, which is measurable on $\cF^{\cK-1}$. By the optimal condition of $\y^*$, we have
$$\nabla_{\cS} f\left(\x^{0}\right) =   -\bH_{\cS} \y^*.$$

Define $\ty^k =  \y^{k} - \y^{*}$. From the update rule of $\y^k$ in \eqref{y update}, we have
\begin{eqnarray}
\bH_{\cS}\ty^k  &=& \nabla g_{\cS}\left( \y^k\right),\label{g ty}\\
\ty^{k+1} &=& \ty^k  - \eta \bH_{\cS} \ty^k. \label{update ty}
\end{eqnarray}
 We can bound the first-order difference of $g_{\cS} \left(\uu^{\sK+1}\right)$ and $g_{\cS} \left(\y^{\sK+1}\right)$ as:
\begin{eqnarray}\label{z8}
&&\< \nabla g_{\cS} \left(\y^{\sK+1}\right),  \uu^{\sK+1} - \y^{\sK+1} \>\overset{\eqref{g ty}}{=}\<\ty^{\sK+1}, \z^{\sK+1} \>_{\bH_{\cS}}\\
&\overset{\eqref{update ty} ~ \eqref{update of z}}{=}& \< (\I -  \eta \bH_{\cS}) \ty^{\sK}  , (\I -  \eta \bH_{\cS})\z^{\sK}  - \eta \bxi_{\uu}^{\sK} -  \eta  \left(\nabla_{\uu} f\left(\x^{\sK}\right) - \nabla g_{\cS}\left(\uu^{\sK}\right)\right)  \>_{\bH_{\cS}}\notag\\
&\overset{a}=& \<\ty^{\sK}, \z^{\sK} \>_{\bH_{\cS} (\I -  \eta \bH_{\cS})^2}  - \eta  \<\ty^{\sK},  \bxi_{\uu}^{\sK}  \>_{\bH_{\cS} (\I -  \eta \bH_{\cS})} - \eta\< \ty^{\sK }, \nabla_{\uu} f\left(\x^{\sK}\right) - \nabla g_{\cS}\left(\uu^{\sK}\right) \>_{\bH_{\cS} (\I -  \eta\bH_{\cS})}\notag\\
&\overset{b}=& - \eta  \sum_{k=0}^{\sK }\<\ty^{k},  \bxi_{\uu}^{k}  \>_{\bH_{\cS} (\I -  \eta \bH_{\cS})^{\sK+1 - k}} - \eta \sum_{k=0}^{\sK }\< \ty^{k}, \nabla_{\uu} f\left(\x^{k}\right) - \nabla g_{\cS}\left(\uu^{k}\right) \>_{\bH_{\cS} (\I -  \eta\bH_{\cS})^{\sK+1 - k}},\notag
\end{eqnarray}
where in $\overset{a} = $, we use $(\I - \bH_{\cS})\bH_{\cS} = \bH_{\cS}(\I - \bH_{\cS})$, and in $\overset{b}=$, we use $\z^{0} = \mathbf{0}$.

We also bound the two terms in the right hand of \eqref{z8}.  For the first term in the right hand of   \eqref{z8},  for all $0\leq k \leq K_0-1$, we have
\begin{eqnarray}\label{z9}
&&\left|\<\ty^{k},  \bxi_{\uu}^{k}  \>_{\bH_{\cS} (\I -  \eta \bH_{\cS})^{\sK+1 - k}}\right|^2=\left|\< \bH_{\cS} \ty^{k},  \bxi_{\uu}^{k}  \>_{ (\I -  \eta \bH_{\cS})^{\sK+1 - k}}\right|^2 \notag\\
&\overset{\eqref{g ty}}{=}& \left|\< \nabla  g_{\cS}\left(\y^k\right),   \bxi_{\uu}^{k} \>_{ (\I -  \eta \bH_{\cS})^{\sK +1- k}}\right|^2\notag\\
&\leq& \sigma^2 \left\|  \nabla  g_{\cS}\left(\y^k\right)\right\|^2 \left\| (\I -  \eta \bH_{\cS})^{\sK - k+1}\right\|_2^2 \leq \sigma^2 \left\|  \nabla  g_{\cS}\left(\y^k\right)\right\|^2.
\end{eqnarray}
So for any $l$ from  $0\leq k \leq K_0-1$,  by standard Azuma–Hoeffding inequality, using $ \nabla  g_{\cS}\left(\y^k\right)$ is measurable on $\cF^{\cK-1}$,  with probability  at least $1-p_3/K_0$,  we have
\begin{eqnarray}\label{protemp}
\left| \eta  \sum_{k=0}^{l}\<\ty^{k},  \bxi_{\uu}^{k}  \>_{\bH_{\cS} (\I -  \eta \bH_{\cS})^{\sK - k}}\right| &\overset{a}{\leq}&  \sqrt{2\eta^2 \sigma^2\log(24K_0/p_3) \sum_{k=0}^{l}\left\|  \nabla  g_{\cS} \left(\y^k\right)\right\|^2 } .
\end{eqnarray}
By union bound, with  probability  at least $1-p_3/12$, \eqref{protemp} holds for all $l$ from $0$ to $K_0-1$. On the other hand, because  $\sK\in [0, K_0-1 ]$, with probability $1-p_3/12$,  we have
\begin{eqnarray}\label{probability3}
\left| \eta  \sum_{k=0}^{\sK}\<\ty^{k},  \bxi_{\uu}^{k}  \>_{\bH_{\cS} (\I -  \eta \bH_{\cS})^{\sK - k}}\right| &\leq&  \sqrt{2\eta^2 \sigma^2\log(24K_0/p_3) \sum_{k=0}^{\sK}\left\|  \nabla  g_{\cS} (\y^k)\right\|^2 } \notag\\
&\overset{a}\leq& \frac{\eta\sum_{k=0}^{\sK}\left\|  \nabla  g_{\cS} (\y^k)\right\|^2  }{16} +8\eta \sigma^2 \log(48/p_3)\log(K_0),
\end{eqnarray}
where  in $\overset{a}\leq$, we use $\sqrt{ab}\leq \frac{a+b}{2}$ with $a\geq0$ and $b\geq0$.

For the second term in the right hand of  \eqref{z8}, we have
\begin{eqnarray}\label{z10}
&&\eta \sum_{k=0}^{\sK }\< \ty^{k}, \nabla_{\uu} f\left(\x^{k}\right) - \nabla g_{\cS}\left(\uu^{k}\right) \>_{\bH_{\cS} (\I -  \eta \bH_{\cS})^{\sK+1 - k}}\notag\\
&=&\eta \sum_{k=0}^{\sK }\<   \nabla  g_{\cS} \left(\y^k\right), \nabla_{\uu} f\left(\x^{k}\right) - \nabla g_{\cS}\left(\uu^{k}\right) \>_{ (\I -  \eta \bH_{\cS})^{\sK+1 - k}}\notag\\
&\leq&\eta \sum_{k=0}^{\sK }\<   \nabla  g_{\cS} \left(\y^k\right), \nabla_{\uu} f\left(\x^{k}\right) - \nabla g_{\cS}\left(\uu^{k}\right) \> \notag\\
&\leq&  \frac{\eta\sum_{k=0}^{\sK}\left\|  \nabla  g_{\cS} \left(\y^k\right)\right\|^2  }{8} + 2\eta  \sum_{k=0}^{\sK}\left\|\nabla_{\uu} f\left(\x^{k}\right) - \nabla g_{\cS}\left(\uu^{k}\right) \right\|^2\notag\\
&\overset{\eqref{basic1}}{\leq}& \frac{\eta\sum_{k=0}^{\sK}\left\|  \nabla  g_{\cS} \left(\y^k\right)\right\|^2  }{8} + \eta \rho^2 B^4 K_0/2.
\end{eqnarray}

Substituting \eqref{probability3} and \eqref{z10} into \eqref{z8}, and using \eqref{z5}, we have
\begin{eqnarray}\label{uu end}
&&g_{\cS}\left(\uu^{\sK+1}\right) \\
&=&  g_{\cS}\left(\y^{\sK+1}\right)+ \< \nabla  g_{\cS}\left(\y^{\sK+1}\right), \uu^{\sK+1} - \y^{\sK+1} \> + \frac{1}{2}\left(\uu^{\sK+1} - \y^{\sK+1}\right)^\bT \bH \left(\uu^{\sK+1} - \y^{\sK+1}\right)\notag\\
&\overset{\eqref{z8}~ \eqref{z5}}\leq&g_{\cS}\left(\y^{\sK+1}\right)+ \frac{3\eta\sum_{k=0}^{\sK}\left\|  \nabla  g_{\cS} (\y^k)\right\|^2  }{16} +4\eta \sigma^2 ( 1+3\log(K_0)) \log(48/p_3) + \rho^2\eta B^4 K_0.\notag
\end{eqnarray}

Then by adding \eqref{uu end} and \eqref{uu end2}, we have
\begin{eqnarray}\label{uu end3}
&&g_{\cS}\left(\uu^{\sK+1}\right)  - g_{\cS} \left(\uu^{0}\right)\notag\\
&\leq&-\frac{25\eta\sum_{k=0}^{\sK}\left\|  \nabla  g_{\cS} \left(\y^k\right)\right\|^2  }{32} +4\eta \sigma^2 ( 1+3\log(K_0)) \log(12/p_3) + \rho^2\eta B^4 K_0.
\end{eqnarray}
\end{proof}

\pb
\begin{proof}[Proofs of Lemma \ref{analysis on vv}]
By the definition of $g_{\cS\bot}(\cdot)$, we have
 \begin{eqnarray}\label{gcs}
 g_{\cS\bot}\left(\vv^{k+1}\right) &=&  g_{\cS\bot}\left(\vv^{k}\right) + \< \nabla g_{\cS\bot}\left(\vv^{k}\right), \vv^{k+1} - \vv^k  \> +  \left[\vv^{k+1} - \vv^{k}\right]^{\bT}\frac{\bH_{\cS\bot}}{2}\left[\vv^{k+1}-\vv^{k}\right]\notag\\
 &\overset{\bH_{\cS\bot}\preceq \mathbf{0}}{\leq}& g_{\cS\bot}\left(\vv^{k}\right) + \< \nabla g_{\cS\bot}\left(\vv^{k}\right) , \vv^{k+1} - \vv^k  \>\notag\\
 &\overset{\eqref{update v}}{=}& g_{\cS\bot}\left(\vv^k\right) -\eta \< \nabla g_{\cS\bot}\left(\vv^{k}\right),   \nabla_{\vv} f\left(\x^{k}\right) + \bxi_{\vv}^k  \>.
 \end{eqnarray}

 We can further bound the right hand of \eqref{gcs} as follows:
 \begin{eqnarray}\label{temp2}
 &&- \< \eta \nabla g_{\cS\bot}\left(\vv^{k}\right),  \nabla_{\vv} f\left(\x^{k}\right)\> \notag\\
 &=& - \eta \left\| \nabla g_{\cS\bot}\left(\vv^{k}\right)  \right\|^2 -  \< \eta \nabla g_{\cS\bot}\left(\vv^{k}\right),  \nabla_{\vv} f(\x^{k})  - \nabla g_{\cS\bot}\left(\vv^{k}\right) \>\notag\\
 &\leq&-   \frac{7\eta}{8}  \left\|\nabla g_{\cS\bot}\left(\vv^{k}\right) \right\|^2 +  2\eta\left\| \nabla_{\vv} f(\x^{k})  - \nabla g_{\cS\bot}\left(\vv^{k}\right) \right\|^2,
 \end{eqnarray}
 where we apply Cauchy Inequality:
 \begin{eqnarray}
  \< \eta\nabla g_{\cS\bot}\left(\vv^{k}\right),  \nabla g_{\cS\bot}\left(\vv^{k}\right)  -   \nabla_{\vv} f\left(\x^{k}\right)\>\leq \frac{\eta \left\| \nabla g_{\cS\bot}\left(\vv^{k}\right)\right\|^2}{8} + 2\eta \left\|\nabla g_{\cS\bot}\left(\vv^{k}\right) - \nabla_{\vv} f\left(\x^k\right) \right\|^2.
 \end{eqnarray}
Substituting \eqref{temp2} into \eqref{gcs},  and telescoping the results with $k$ from $0$ to $\sK$,  we have
 \begin{eqnarray}\label{g_vv end}
 &&g_{\cS\bot}\left(\vv^{\sK+1}\right) \\
  &\leq&g_{\cS\bot}\left(\vv^{0}\right)  -  \sum_{k =0}^{\sK}  \eta\< \nabla g_{\cS\bot}\left(\vv^{k}\right),  \bxi_{\vv}^k\>  - \frac{7\eta}{8}\sum_{k =0}^{\sK}  \left\|  \nabla g_{\cS\bot}\left(\x^{k}\right)  \right\|^2+2\eta\sum_{k =0}^{\sK}\left\| \nabla_{\vv} f\left(\x^{k}\right)  - \nabla g_{\cS\bot}\left(\vv^{k}\right) \right\|^2\notag\\
 &\leq&g_{\cS\bot}\left(\vv^{0}\right)  -  \sum_{k =0}^{\sK}  \eta\< \nabla g_{\cS\bot}\left(\vv^{k}\right),  \bxi_{\vv}^k\>  - \frac{7\eta}{8}\sum_{k =0}^{\sK}  \left\|  \nabla g_{\cS\bot}\left(\x^{k}\right)  \right\|^2 + \frac{\rho^2 B^4 \eta K_0}{2}.\notag
 \end{eqnarray}

\end{proof}

\pb\subsection{Proof of Theorem \ref{faster descent}}
Because whether $\x^{k}$ goes out of the neighborhood of $\x^{0}$ in $K_0$ steps cannot be predicable given $\cF^{\cK-1}$, to bound  $ \sum_{k =0}^{\sK}  \eta\< \nabla g_{\cS\bot}\left(\vv^{k}\right),  \bxi_{\vv}^k\>$, we consider  the following two cases:
\begin{enumerate}
	\item $\left\|\nabla f\left(\x^{0}\right)\right\|> 5 \sigma$,\label{case11}
	\item $\left\|\nabla f\left(\x^{0}\right)\right\|\leq 5 \sigma$. \label{case12}
\end{enumerate}
For the first case, the function value is guaranteed to decrease monotonously. For the second case, we  bound  $ \sum_{k =0}^{\sK}  \eta\< \nabla g_{\cS\bot}(\vv^{k}),  \bxi_{\vv}^k\>$ by concentration laws.

\pb
\noindent\textbf{Case \ref{case11}:} If  $\left\|\nabla f_\vv\left(\x^{0}\right)\right\|> 5 \sigma$,  we have, for all $0\leq k \leq \sK(j)$,
\begin{eqnarray}\label{boundna}
\left\|\nabla f\left(\x^{k}\right) \right\|\geq \left\| \nabla f\left(\x^{0}\right) \right\| - \left\|\nabla f\left(\x^{k}\right)-  \nabla f\left(\x^{0}\right) \right\|\geq 5\sigma - L B \geq \frac{9}{2} \sigma.
\end{eqnarray}
We need $LB\leq \frac{1}{2}$.
Thus for $f(\cdot)$ has Lipschitz gradients, we have for all $0\leq k \leq \sK(j)$, we have 
\begin{eqnarray}\label{case1all}
&&f\left(\x^{k+1}\right)-f\left(\x^{k}\right) \notag\\
&\leq& \< \nabla f\left(\x^{k}\right),\x^{k+1} - \x^{k}  \> + \frac{L}{2}\| \x^{k+1} - \x^{k}\|^2\notag\\
&\leq&  -\eta \left\| \nabla f\left(\x^{k}\right) \right\|^2 - \eta  \< \nabla f\left(\x^{k}\right) , \bxi^{k}\> + L\eta^2\left\| \nabla f\left(\x^{k}\right) \right\|^2 + L \eta^2\sigma^2\notag\\
&\overset{a}{\leq}& -\frac{15\eta}{16}\left\| \nabla f\left(\x^{k}\right) \right\|^2 +\frac{5\eta}{32}\left\| \nabla f\left(\x^{k}\right) \right\|^2 + \frac{8}{5} \eta \sigma^2 + L\eta^2 \sigma^2\notag\\
&\leq& -\frac{25\eta}{32}\left\| \nabla f\left(\x^{k}\right) \right\|^2 +2\eta\sigma^2\overset{\eqref{boundna}}{\leq} - \eta\left(\frac{25}{32} - \frac{8}{81}\right)\left\| \nabla f\left(\x^{k}\right) \right\|^2,
\end{eqnarray}
where in $\overset{a}\leq$, we use $L\eta\leq \frac{1}{16}$ from \eqref{parametersetting} and $-\< \nabla f\left(\x^{k}\right) , \bxi^{k}\> \leq \frac{5}{32} \left\| \nabla f\left(\x^{k}\right) \right\|^2+ \frac{8}{5}\left\|\bxi^k \right\|^2$.

By telescoping \eqref{case1all} with $k$ from $0$ to $\sK$, we have
\begin{eqnarray}
&&f\left(\x^{\cK(j+1)}\right)-f\left(\x^{0}\right)  \leq  - \eta\left(\frac{25}{32} - \frac{8}{81}\right) \sum_{k=0}^{\sK(j)}\left\| \nabla f\left(\x^{k}\right) \right\|^2.
\end{eqnarray}
On the other hand, we have
\begin{eqnarray}
&&\left\| \eta \sum_{k=0}^{\sK(j)} \nabla f\left(\x^{k}\right)  \right\|=\left\| -\eta \sum_{k=0}^{\sK(j)} \nabla f\left(\x^{k}\right)  \right\|\notag\\
&=& \left\| \x^{\sK(j)+1} - \x^{0} + \eta \sum_{k=0}^{\sK(j)}\xi^k  \right\|\notag\\
&\geq& \left\| \x^{\sK(j)+1} - \x^{0}\right\| - \left\| \eta \sum_{k=0}^{\sK(j)}\xi^k  \right\|.
\end{eqnarray}
 By the Vector-Martingale Concentration Inequality in Subsection \ref{123}, we have with probability $1 - p_3/12$,  
\begin{eqnarray}\label{tempp}
\left\| \sum_{k=0}^{\sK(j)} \bxi^k  \right\|\leq 2\eta \sigma\sqrt{ (\sK +1) \log(48/p_3)} \leq 2\eta \sigma\sqrt{ K_0 \log(48/p_3)} \leq \frac{B}{16}.
\end{eqnarray} 
So on the event  $\x^k$ exits $\cB\left(\x^{0},B\right)$ in $K_0$ iterations, and \eqref{tempp} happens, we have
\begin{eqnarray}
&&\eta \sum_{k=0}^{\sK(j)}\left\| \nabla f\left(\x^{k}\right) \right\|^2 \notag\\ 
&\overset{a}{\geq}&  \frac{1}{ \eta(\sK(j) )+\eta}\left\| \eta\sum_{k=0}^{\sK(j)}  \nabla f\left(\x^{k}\right) \right\|^2 \geq    \frac{1}{ \eta(\sK(j) )+\eta} \left(B - \frac{1}{16}B\right)^2\notag\\
&\geq&\frac{15^2B^2}{16^2 \eta(\sK(j)  +1)}\overset{\sK(j) +1 \leq K_0}{\geq} \frac{15^2B^2}{16^2\eta K_0},
\end{eqnarray}
where in $\overset{a}\geq$, we use the inequality  that 
$$ \left\|\sum_{i=1}^l \a_i \right\|^2 \leq l \sum_{i=1}^l \left\|\a_i\right\|^2,  $$
holds for all $l\geq 1$. We obtain
\begin{eqnarray}
f\left(\x^{\cK(j+1)}\right) &\leq&  f\left(\x^{0}\right)  - \left(\frac{25}{32} - \frac{8}{81}\right) \frac{15^2B^2}{16^2\eta K_0} \notag\\
& \leq&  f\left(\x^{0}\right)  -\frac{B^2}{7\eta K_0}.
\end{eqnarray}

\pb
\noindent\textbf{Case \ref{case12}:}   Because  $\left\|\nabla f_\vv\left(\x^{0}\right)\right\|\leq \left\|\nabla f\left(\x^{0}\right)\right\|\leq 5 \sigma$,  we have, for all $\cK\leq k \leq \sK(j)$, 
\begin{eqnarray}\label{boundnabla}
\left\|\nabla g_{\cS\bot}\left(\vv^{k}\right) \right\|\leq \left\| \nabla g_{\cS\bot}\left(\vv^{0}\right) \right\| + \left\|\nabla g_{\cS\bot}\left(\vv^{k}\right)- \nabla g_{\cS\bot}\left(\vv^{0}\right) \right\|\leq 5\sigma + L B \leq \frac{11}{2} \sigma.
\end{eqnarray}
In the same way, we also have
\begin{eqnarray}
\left\|\nabla f\left(\x^{\sK(j)}\right) \right\|\leq \frac{11\sigma}{2},
\end{eqnarray}
which indicates that
\begin{eqnarray}\label{xbound}
\left\|\x^{\cK(j+1)} - \x^{0} \right\| \leq \left\| \x^{\cK(j+1)} -\x^{\sK(j)} \right\|+ \left\|\nabla f\left(\x^{\sK(j)}\right) + \bxi^{\sK(j)}\right\| \leq B + \frac{13}{2}\eta \sigma \overset{\eqref{parametersetting}}{\leq} B+\frac{B}{100}.  
\end{eqnarray}

Then by adding \eqref{uu end3} and \eqref{g_vv end}, and using  $\rho$-smoothness of Hessian, i.e.,
\begin{eqnarray}
f\left(\x^{\cK(j+1)}\right) - f\left(\x^{0}\right) - g_{\cS}\left(\uu^{\cK(j+1)}\right) - g_{\cS\bot}\left(\vv^{\cK(j+1)}\right)     \leq \frac{\rho}{6}\|\x^{\cK(j+1)} - \x^{0} \|^3 \overset{\eqref{xbound}}{\leq}  \frac{\rho B^3}{5},
\end{eqnarray}
and $ g_{\cS}\left(\uu^{0}\right) + g_{\cS\bot}\left(\vv^{0}\right)=0$, we have
\begin{eqnarray}\label{end22}
&&f\left(\x^{\cK(j+1)}\right) \\
&\leq& f\left(\x^{0}\right)  -   \eta\sum_{k =0}^{\sK(j)} \<  \nabla g_{\cS\bot}\left(\vv^{k}\right),  \bxi_{\vv}^k\> + 4\eta \sigma^2 \left( 1+3\log(K_0)\right) \log(48/p_3)\notag\\
&& - \frac{7\eta}{8} \sum_{k =0}^{\sK(j)}  \left\| \nabla g_{\cS\bot}\left(\vv^{k}\right)  \right\|^2 -\frac{25\eta  }{32} \sum_{k=0}^{\sK(j)}\left\|  \nabla  g_{\cS} \left(\y^k\right)\right\|^2 + \frac{3\rho^2 B^4 \eta K_0}{2} +\frac{\rho B^3}{5}. \notag
\end{eqnarray}

With the parameter set in \eqref{parametersetting}, we have
\begin{eqnarray}
4\eta \sigma^2 \left( 1+3\log(K_0)\right) \log(48/p_3) \leq  \frac{B^2}{256\eta K_0},
\end{eqnarray}
\begin{eqnarray}
\frac{3\rho^2 B^4 \eta K_0}{2}  \leq  \frac{B^2}{128\eta K_0},
\end{eqnarray}
and
\begin{eqnarray}
\frac{\rho B^3}{5} \leq  \frac{B^2}{80\eta K_0},
\end{eqnarray}
so
\begin{eqnarray}\label{end2}
f\left(\x^{\cK(j+1)}\right)&\leq& f\left(\x^{0}\right)  -  \eta\sum_{k =0}^{\sK(j)}  \<  \nabla g_{\cS\bot}\left(\vv^{k}\right),  \bxi_{\vv}^k\> + \left(\frac{3}{256}+ \frac{1}{80}\right) \frac{B^2}{\eta K_0}\notag\\
&& - \frac{7\eta}{8}  \sum_{k =0}^{\sK(j)}  \left\| \nabla g_{\cS\bot}\left(\vv^{k}\right)  \right\|^2 -\frac{25\eta\sum_{k=0}^{\sK(j)}\left\|  \nabla  g_{\cS} \left(\y^k\right)\right\|^2  }{32}. \notag
\end{eqnarray}

\redd{ We define the following random stopping times:
\begin{eqnarray}\label{probability6}
\tau^l = \min\left(\inf\left(\sum_{k = \tau^{l-1}+1}^{\tau^{l}+1} \eta\left(\left\| \nabla g_{\cS\bot}\left(\vv^k\right)\right\|^2+ \left\| \nabla g_{\cS}\left(\y^k\right)\right\|^2\right)\geq  \frac{169B^2}{512\eta K_0}\right), K_0-1 \right), ~ 1\leq l\leq K_0.
\end{eqnarray}
with $\tau^0 =0-1$.}

\redd{Our result is based on the following events happens:
\begin{eqnarray}\label{end1}
\left\|\sum_{k = \tau^{l-1}+1}^{\tau^l }\eta\< \nabla g_{\cS\bot}\left(\vv^k\right), \bxi^k_\vv \>\cI_{k\leq \sK(j)}\right\| \leq \sigma\sqrt{ \frac{169B^2}{128 K_0}\log(3K_0/p_3) },  ~ 1\leq l \leq K_0.
\end{eqnarray}
where $\cI$ denotes the indication function.}

\redd{Then from the definition  of $\tau^l$, we have for all $l$ from $1$ to $K_0$,
\begin{eqnarray}
&&\sum_{k = \tau^{l-1}+1}^{\tau^l} \E \left[\left\|\eta\< \nabla g_{\cS\bot}\left(\vv^k\right), \bxi^k_\vv \>\cI_{k\leq \sK(j)}\right\|^2\mid \cF^{k-1}\right]\notag\\
&\overset{a}\leq&\sum_{k = \tau^{l-1}+1}^{\tau^l} \E \left[\left\|\eta\< \nabla g_{\cS\bot}\left(\vv^k\right), \bxi^k_\vv \>\right\|^2\mid \cF^{k-1}\right]\left\|\cI_{k\leq \sK(j)}\right\|^2\notag\\
&\leq& \sum_{k = \tau^{l-1}+1}^{\tau^l} \eta^2 \left\|g_{\cS\bot}\left(\vv^k\right) \right\|^2 \E \left[\left\| \bxi^k_\vv \right\|^2\mid \cF^{k-1}\right]\left\|\cI_{k\leq \sK(j)}\right\|^2  \notag\\
&\leq& \sum_{k = \tau^{l-1}+1}^{\tau^l} \eta^2 \left\|\nabla g_{\cS\bot}\left(\vv^k\right) \right\|^2\sigma^2 \leq  \frac{169B^2\sigma^2}{512K_0},\notag
\end{eqnarray}
where in $\overset{a}\leq$, we use $\cI_{ \sK(j) \geq k}=\cI_{ \sK(j) > k-1}$ is measurable on $\cF^{K-1}$.}

\redd{Also from \eqref{boundnabla},  we have $\left\| \eta\< \nabla g_{\cS\bot}\left(\vv^k\right), \bxi^k_\vv \>\cI_{k\leq \cK(j+1)}\right\| \leq \eta \sigma (5\sigma +LB) \leq 6\eta \sigma^2.$ Thus by Berinstein inequality in Theorem \cite{}????, for any $1\leq l \leq K_0$, we have
\begin{eqnarray}\label{133}
&&\PP\left(\left\|\sum_{k = \tau^{l-1}}^{\tau^l -1}\eta\< \nabla g_{\cS\bot}\left(\vv^k\right), \xi^k_\vv \>\right\| \geq \sigma\sqrt{ \frac{169B^2}{128 K_0}\log(3K_0/p_3) }\right)\notag\\
&\leq& \exp\left(-   \frac{\sigma^2 \frac{169B^2}{128 K_0}\log\left(3K_0/p_3\right)}{   2\sigma^2  \frac{169B^2}{512 K_0} + 2\cdot 6\eta\sigma  \sqrt{ \frac{169B^2}{256 K_0}\log\left(3K_0/p_3\right) }  } \right).
\end{eqnarray}}

With the parameter set in \eqref{parametersetting}, we have
\begin{eqnarray}
6\eta\sigma^2  \sqrt{ \frac{169B^2}{256 K_0}\log(3K_0/p_3) } \leq   \sigma^2   \frac{169B^2}{512 K_0},
\end{eqnarray}
and 
\begin{eqnarray}
\sigma\sqrt{ \frac{169B^2}{128 K_0}\log\left(3K_0/p_3\right) }\leq \frac{B^2}{25\eta K_0}.
\end{eqnarray}

\redd{So by union bound, \eqref{end1} happens with probability at least $\frac{1}{3}p_3$. On the other hand, for all $l$ from $1$ to $K_0$, we have
\begin{eqnarray}\label{qwe}
\left\|\eta\< \nabla g_{\cS\bot}\left(\vv^{\tau^l}\right), \bxi^{\tau^l}_\vv \> \cI_{k\leq \sK(j)}\right\|\leq\frac{\eta\left\| \nabla g_{\cS\bot}\left(\vv^{\tau^l}\right)\right\|^2}{16} \cI_{k\leq \sK(j)}+ 4\eta \sigma^2 \cI_{k\leq \sK(j)}. 
\end{eqnarray}}

\redd{Let
\begin{eqnarray}
\sK_2 = \sup_{l\leq K_0}\left(\tau^{l} \leq \sK(j)\right),
\end{eqnarray}
we have
\begin{eqnarray}\label{end4}
&&f\left(\x^{\cK(j+1)}\right)  - f\left(\x^{0}\right)\notag\\
 &\leq&   -  \sum_{l=1}^{\sK_2}\left(\sum_{k = \tau^{l-1}+1}^{\tau^{l}} \left( \eta\<  \nabla g_{\cS\bot}\left(\vv^{k}\right),  \bxi_{\vv}^k\> - \frac{7\eta}{8}  \left\| \nabla g_{\cS\bot}\left(\vv^{k}\right)  \right\|^2 -\frac{25\eta\left\|  \nabla  g_{\cS} \left(\y^k\right)\right\|^2  }{32} \right)\right) \notag\\
&&  - \sum_{k = \sK_2}^{\sK}\left(  \eta\<  \nabla g_{\cS\bot}\left(\vv^{k}\right),  \bxi_{\vv}^k\> - \frac{7\eta}{8}    \left\| \nabla g_{\cS\bot}\left(\vv^{k}\right)  \right\|^2 -\frac{25\eta\left\|  \nabla  g_{\cS} \left(\y^k\right)\right\|^2  }{32} \right)\notag\notag\\
&&+ \left(\frac{3}{256}+ \frac{1}{80}\right) \frac{B^2}{\eta K_0}\notag\\
&\overset{\eqref{qwe}}\leq&   -  \sum_{l=1}^{\cK_2}\left(\sum_{k = \tau^{l-1}+1}^{\tau^{l}-1} \eta\<  \nabla g_{\cS\bot}\left(\vv^{k}\right),  \bxi_{\vv}^k\>  - \frac{25\eta}{32}\sum_{k = \tau^{l-1}+1}^{\tau^{l}}\left(   \left\| \nabla g_{\cS\bot}\left(\vv^{k}\right)  \right\|^2 +\left\|  \nabla  g_{\cS} \left(\y^k\right)\right\|^2  \right) +4\eta \sigma^2\right) \notag\\
&&   - \sum_{k = \sK_2}^{\sK}\left(  \eta\<  \nabla g_{\cS\bot}\left(\vv^{k}\right),  \bxi_{\vv}^k\> - \frac{7\eta}{8}    \left\| \nabla g_{\cS\bot}\left(\vv^{k}\right)  \right\|^2 -\frac{25\eta\left\|  \nabla  g_{\cS} \left(\y^k\right)\right\|^2  }{32} \right)\notag\notag\\
&&+ \left(\frac{3}{256}+ \frac{1}{80}\right) \frac{B^2}{\eta K_0}\notag\\
&\leq& -(\sK_2)\left(  \frac{25}{32}\cdot\frac{169B^2}{512\eta K_0}  -4\eta\sigma^2 - \frac{B^2}{25\eta K_0}\right) + \left(\frac{3}{256}+ \frac{1}{80}+ \frac{1}{25}\right) \frac{B^2}{\eta K_0}\notag\\
&\leq&+ \left(\frac{3}{256}+ \frac{1}{80}\right) \frac{B^2}{\eta K_0}\notag\\
&\leq& -(\sK_2)\left(  \frac{25}{32}\cdot\frac{169B^2}{512\eta K_0} - \frac{B^2}{128\eta K_0}  - \frac{B^2}{25\eta K_0}\right) + \left(\frac{3}{256}+ \frac{1}{80}+ \frac{1}{25}\right) \frac{B^2}{\eta K_0}.
\end{eqnarray}}

At last, we prove with high probability, $\cK_2\geq1$. Considering
\begin{eqnarray}
&&\left\|\eta\sum_{k=0}^{\sK(j)}  \left(\nabla g_{\cS\bot}\left(\vv^{k}\right) +  \nabla g_{\cS} \left(\y^k\right)\right) \right\|=\left\|-\eta\sum_{k=0}^{\sK(j)}  \left(\nabla g_{\cS\bot}\left(\vv^{k}\right) +  \nabla g_{\cS} \left(\y^k\right)\right) \right\|\notag\\
&=&\left\|\vv^{\cK(j+1)} - \vv^{0}   + \eta\sum_{k=0}^{\sK(j)} \left(\bxi_{\vv}^k-  \nabla g_{\cS\bot} (\x^k)  + \nabla f_{\vv}(\x^k)\right)  + \y^{\cK(j+1)} - \y^{0} \right\|\notag\\
&\geq&\left\|  \vv^{\cK(j+1)}  - \vv^{0}  + \eta\sum_{k=0}^{\sK(j)} \bxi_{\vv}^k   +  \left(\uu^{\cK(j+1)} - \uu^{0}\right) -\left( \z^{\cK(j+1)} - \z^{0}\right)   \right\|\notag\\ &&-\left\|\eta \sum_{k=0}^{\sK(j)} \left(\nabla g_{\cS\bot} \left(\x^k\right)  - \nabla f_{\vv}\left(\x^k\right)\right) \right\| \notag\\
&\geq&\left\|  \x^{\cK(j+1)}  - \x^{0}\right\|   - \left\|\z^{\cK(j+1)} - \z^{0} \right\| -\eta \left\| \sum_{k=0}^{\sK(j)} \bxi_{\vv}^k  \right\| - \frac{\eta K_0 \rho B}{2}\notag\\
&\overset{\eqref{z4}}\geq&\left\|  \x^{\cK(j+1)}  - \x^{0}\right\| - \frac{3B}{32} -\frac{B}{32} - \eta \left\| \sum_{k=0}^{\sK(j)} \bxi_{\vv}^k \right\|. 
\end{eqnarray}
Like \eqref{probability1}, by the Vector-Martingale Concentration Inequality in Subsection \ref{123}, we have with probability $1 - p_3/12$,  
\begin{eqnarray}\label{probability4}
\left\| \sum_{k=0}^{\sK(j)} \bxi_{\vv}^k \right\|\leq 2\eta \sigma\sqrt{ (\sK +1) \log(48/p_3)} \leq 2\eta \sigma\sqrt{ K_0 \log(48/p_3)} \leq \frac{B}{16}.
\end{eqnarray} 
We obtain
\begin{eqnarray}\label{2end2}
\left\|\eta\sum_{k=0}^{\sK(j)}  \left( \nabla f_{\vv} \left(\vv^k\right) +  \nabla g_{\cS} \left(\y^k\right)\right)\right\|\geq\left\|  \x^{\cK(j+1)}  - \x^{0}\right\| - \frac{3B}{16}. 
\end{eqnarray}
So on the event  $\x^k$ exits $\cB\left(\x^{0},B\right)$ in $K_0$ iterations,  with probability $1-p_3/3$ (\eqref{probability1}, \eqref{probability2}, \eqref{probability3} and \eqref{probability4} happen), we  have
\begin{eqnarray}\label{2endim}
&&\eta \sum_{k = \sK(j)}^{\sK(j)}  \left\| \nabla g_{\cS\bot}\left(\x^{k}\right)  \right\|^2+\eta\sum_{k=0}^{\sK(j)}\left\|  \nabla  g_{\cS} \left(\y^k\right)\right\|^2 \notag\\ 
&\overset{a}{\geq}&  \frac{1}{2 \eta(\sK(j) )+\eta}\left\| \eta \sum_{k =0}^{\sK(j)-1} \left(  \nabla g_{\cS\bot}\left(\x^{k}\right)  +   \nabla  g_{\cS} \left(\y^k\right)\right)  +  \eta \nabla f(\x^{\sK(j)-1}) \right\|^2 \notag\\
&\overset{\eqref{2end2}}{\geq}&\frac{169B^2}{512 \eta(\sK(j)  +1)}\overset{\sK(j) +1 \leq K_0}{\geq} \frac{169B^2}{512\eta K_0},
\end{eqnarray}
which indicates that $\cK_2\geq1$.

In all, under the events   $\x^k$ exits $\x^{0}$ in $K_0$ iterations happens, with probability at least $\frac{2}{3}p_3$ (\eqref{probability1}, \eqref{probability2}, \eqref{probability3}, \eqref{probability4}, and \eqref{probability6} happen),  from \eqref{end4}, and $\cK_2 \geq 1$, we have
\begin{eqnarray}
f\left(\x^{\cK(j+1)}\right)  - f\left(\x^{0}\right)\leq -\left(  \frac{25}{32}\cdot\frac{169}{512} - \frac{1}{128}  - \frac{1}{25} -\frac{3}{256}- \frac{1}{80}- \frac{1}{25} \right) \frac{B^2}{\eta K_0}\leq -\frac{B^2}{7\eta K_0}.
\end{eqnarray}

Combining Case \ref{case11} and Case \ref{case12}, we obtain Theorem \ref{faster descent}.
